# Supplementary material for: $\texttt{SPIN}$: distilling $\texttt{Skill-RRT}$ for long-horizon prehensile and non-prehensile manipulation
Source: arXiv:2502.18015 source file (2025-05-07)
Supplement: Supplementary file 1 [file P_action.tex]

\begin{table}[H]
\centering
\caption{Action Information for NP skill Policy}\label{table:P_action}
% \begin{adjustbox}{width=0.5\textwidth} % Scales the table to half the page width
\begin{tabular}{|c|c|} % Adjust the last column width to fit half-page format
\hline
\textbf{Symbol} & \textbf{Description}  \\
\hline
$\Delta q_\text{ee}\in\mathbb{R}^6$& \text{Delta end-effector pose} \\ \hline
$k_p\in\mathbb{R}^7$ & \text{proportional gain}   \\ \hline
$\rho\in\mathbb{R}^7$ & \text{joint damping}  \\ \hline
\end{tabular}
% \end{adjustbox}
\end{table}
