# Supplementary material for: $\texttt{SPIN}$: distilling $\texttt{Skill-RRT}$ for long-horizon prehensile and non-prehensile manipulation
Source: arXiv:2502.18015 source file (2025-05-07)
Supplement: Supplementary file 2 [file Baseline_MAPLE_state.tex]

\begin{table}[H]
\centering
% \begin{adjustbox}{width=0.5\textwidth}
\begin{tabular}{|c|c|}
\hline
 \textbf{Symbol} & \textbf{Description} \\ \hline
$q^\text{(t)}_r \in \mathbb{R}^9$ &robot joint position  \\ \hline

$\dot{q}^\text{(t)}_r \in \mathbb{R}^9$ &robot joint velocity  \\ \hline

$p^\text{(t)}_\text{ee} \in \mathbb{R}^{24}$ & robot end-effector keypoint positions. \\ \hline

$p^\text{(t)}_\text{tip} \in \mathbb{R}^6$ & Robot gripper tip positions \\ \hline

$p^\text{(t)}_\text{ee-rel} \in \mathbb{R}^{24}$ & \makecell{relative robot end-effector \\ keypoint positions w.r.t $q^\text{(t)}_\text{obj}$}. \\ \hline

$p^\text{(t)}_\text{tip-rel} \in \mathbb{R}^6$ & \makecell{relative robot gripper \\ tip positions  w.r.t $q^\text{(t)}_\text{obj}$} \\ \hline

$p^\text{(t)}_\text{obj} \in \mathbb{R}^{24}$ &object keypoint positions  \\ \hline

$p^\text{g}_\text{obj} \in \mathbb{R}^{24}$ &target object keypoint positions \\ 
\hline
\end{tabular}
% \end{adjustbox}
\vspace{-0.2cm}
\caption{The components of state space $S$ of the baseline MAPLE policy.}\label{table:Maple_state}
\end{table}
