# Supplementary material for: $\texttt{SPIN}$: distilling $\texttt{Skill-RRT}$ for long-horizon prehensile and non-prehensile manipulation
Source: arXiv:2502.18015 source file (2025-05-07)
Supplement: Supplementary file 4 [file Baseline_PPO_state.tex]

\begin{table}[h]
\centering
% \begin{adjustbox}{width=0.5\textwidth}
\caption{State configuration of the baseline PPO policy.}\label{table:PPO_state}
\begin{tabular}{|c|c|c|}
\hline
\textbf{Extract From} &  \textbf{Symbol} & \textbf{Description} \\
\hline
\multirow{4}{*}{Robot configuration}& $q^\text{(t)}_r \in \mathbb{R}^9$ &Robot joint position  \\
\cline{2-3}
& $\dot{q}^\text{(t)}_r \in \mathbb{R}^9$ &Robot joint velocity  \\
\cline{2-3}
&  $p^\text{(t)}_\text{ee} \in \mathbb{R}^{24}$ & Robot end-effector keypoint positions. \\
\cline{2-3}
&  $p^\text{(t)}_\text{tip} \in \mathbb{R}^6$ & Robot gripper tip positions \\
\hline
\multirow{2}{*}{Robot and object configuration}& $p^\text{(t)}_\text{ee-rel} \in \mathbb{R}^{24}$ & \makecell{Relative robot end-effector \\ keypoint positions w.r.t $q^\text{(t)}_\text{obj}$}. \\
\cline{2-3}
&  $p^\text{(t)}_\text{tip-rel} \in \mathbb{R}^6$ & \makecell{Relative robot gripper \\ tip positions  w.r.t $q^\text{(t)}_\text{obj}$} \\
\hline
Object configuration&  $p^\text{(t)}_\text{obj} \in \mathbb{R}^{24}$ &Object keypoint positions  \\
\hline
Target object pose & $p^\text{g}_\text{obj} \in \mathbb{R}^{24}$ &Target object keypoint positions \\
\hline
Action & $a^\text{(t-1)} \in \mathbb{R}^{21}$ &Previous action \\
\hline
\end{tabular}
% \end{adjustbox}
\vspace{-0.2cm}
\begin{flushleft}
\footnotesize
\end{flushleft}
\end{table}
