# Supplementary material for: $\texttt{SPIN}$: distilling $\texttt{Skill-RRT}$ for long-horizon prehensile and non-prehensile manipulation
Source: arXiv:2502.18015 source file (2025-05-07)
Supplement: Supplementary file 5 [file region_params.tex]

\begin{table}[H]
\centering
\setlength\tabcolsep{20 pt}

\caption{Real value of region parameters. $x, y, h, l$ are in $m$, and $\theta$ is in $rad$.}\label{table:region_params}
% \begin{adjustbox}{width=\textwidth} % Adjusts the table width to half the page
\begin{tabular}{|c|c|c|c|c|c|}
\hline
\multicolumn{6}{|c|}{\textbf{Card Flip}} \\ 
\hline
$x^{\text{table}}_{\text{min}}$ & $x^{\text{table}}_{\text{max}}$ & $y^{\text{table}}_{\text{min}}$ & $y^{\text{table}}_{\text{max}}$ &  & \\
\hline
$0.35$ & $0.65$ & $-0.15$ & $0.15$ &  & \\
\hline
\multicolumn{6}{|c|}{\textbf{Bookshlef}} \\ 
\hline
$l_{\text{book}}$ & $h_{\text{book}}$ & $\theta^{\text{uppershelf}}_{\text{max}}$ & & & \\
\hline
$0.07$ & $0.1$ & $\pi/4$ & $ $ & $ $ & $ $ \\
\hline
$x^{\text{lowershelf}}_{\text{min}}$ & $x^{\text{lowershelf}}_{\text{max}}$ & $y^{\text{lowershelf}}_{\text{min}}$ & $y^{\text{lowershelf}}_{\text{max}}$ & $\theta^{\text{lowershelf}}_{\text{min}}$ & $\theta^{\text{lowershelf}}_{\text{max}}$ \\
\hline
$0.67$ & $0.76$ & $-0.08$ & $0.08$ & $-\pi/20$ & $\pi/20$ \\
\hline
\multicolumn{6}{|c|}{\textbf{Kitchen}} \\ 
\hline
$x^{\text{l-cupboard}}_{\text{min}}$ & $x^{\text{l-cupboard}}_{\text{max}}$ & $y^{\text{l-cupboard}}_{\text{min}}$ & $y^{\text{l-cupboard}}_{\text{max}}$ & $\theta^{\text{l-cupboard}}_{\text{min}}$ & $\theta^{\text{l-cupboard}}_{\text{max}}$ \\
\hline
$0.5585$ & $0.6285$ & $0.2205$ & $0.2805$ & $5\pi/6$ & $7\pi/6$ \\
\hline
$x^{\text{r-cupboard}}_{\text{min}}$ & $x^{\text{r-cupboard}}_{\text{max}}$ & $y^{\text{r-cupboard}}_{\text{min}}$ & $y^{\text{r-cupboard}}_{\text{max}}$ & $\theta^{\text{r-cupboard}}_{\text{min}}$ & $\theta^{\text{r-cupboard}}_{\text{max}}$ \\
\hline
$0.5585$ & $0.6285$ & $-0.2805$ & $-0.2205$ & $5\pi/6$ & $7\pi/6$ \\
\hline
\end{tabular}
% \end{adjustbox}
\end{table}
